# Supplementary material for: Many-body interferometry with semiconductor spins
Source: arXiv:2511.04310 source file (2025-11-06)

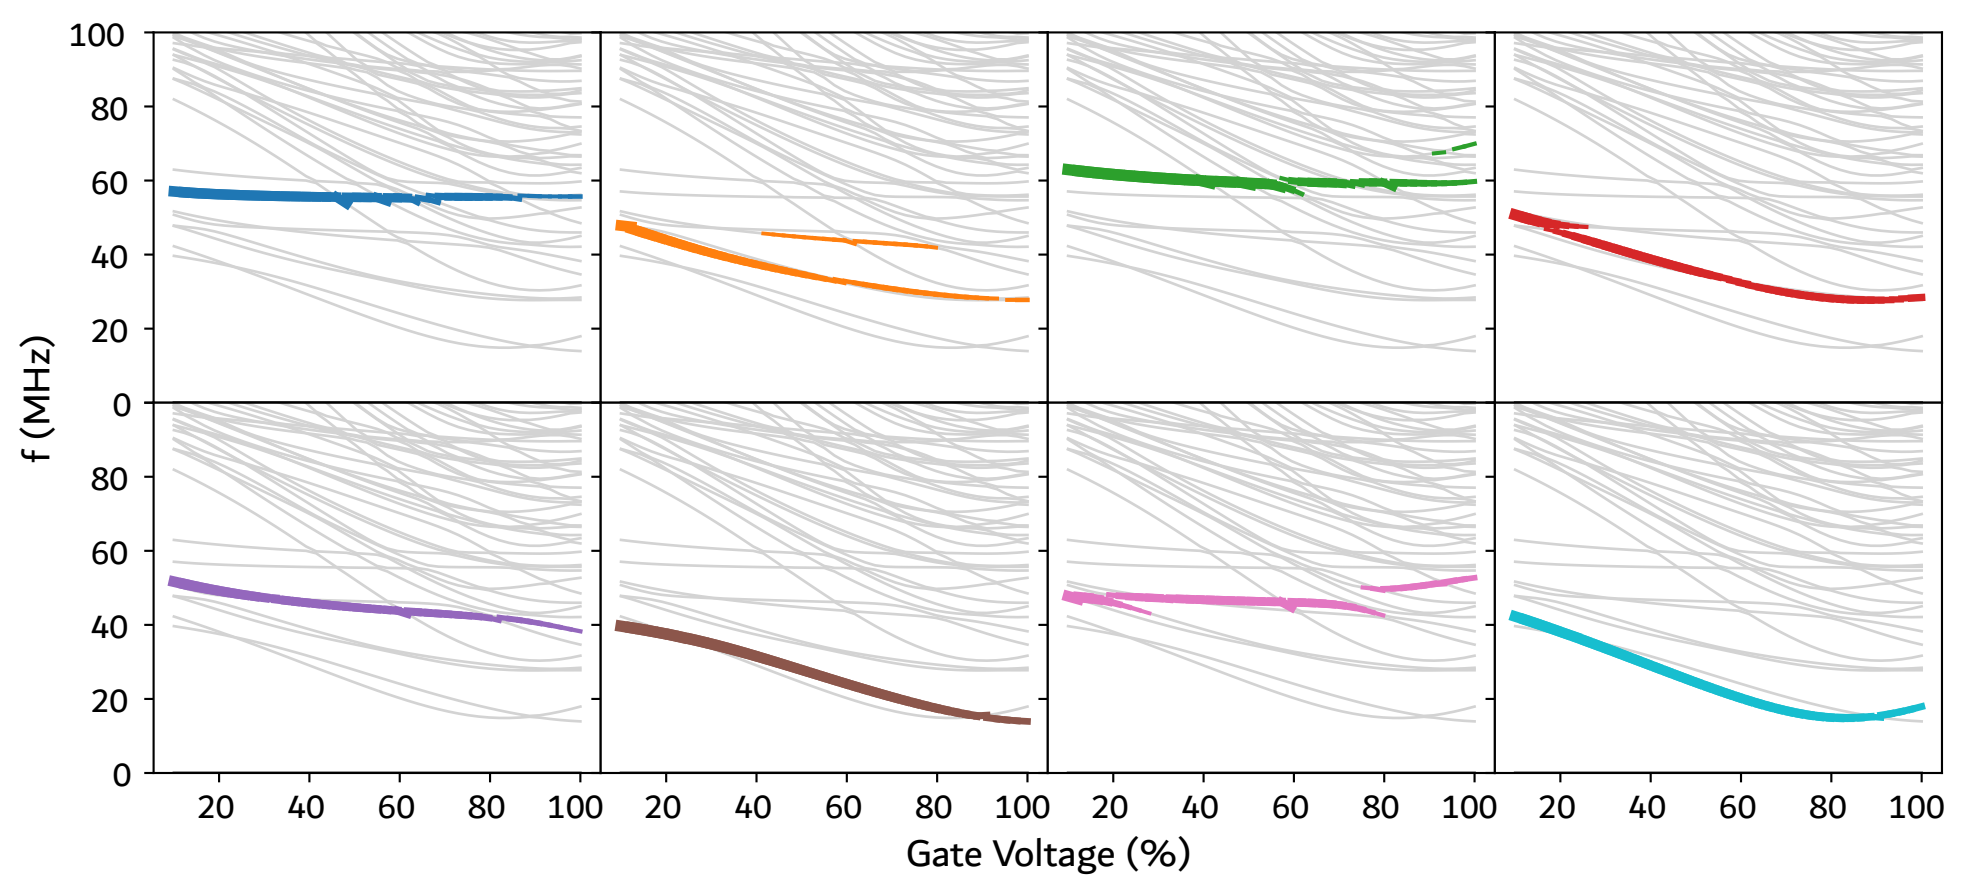

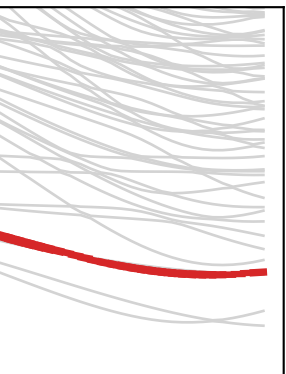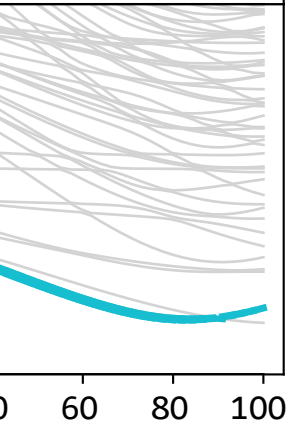

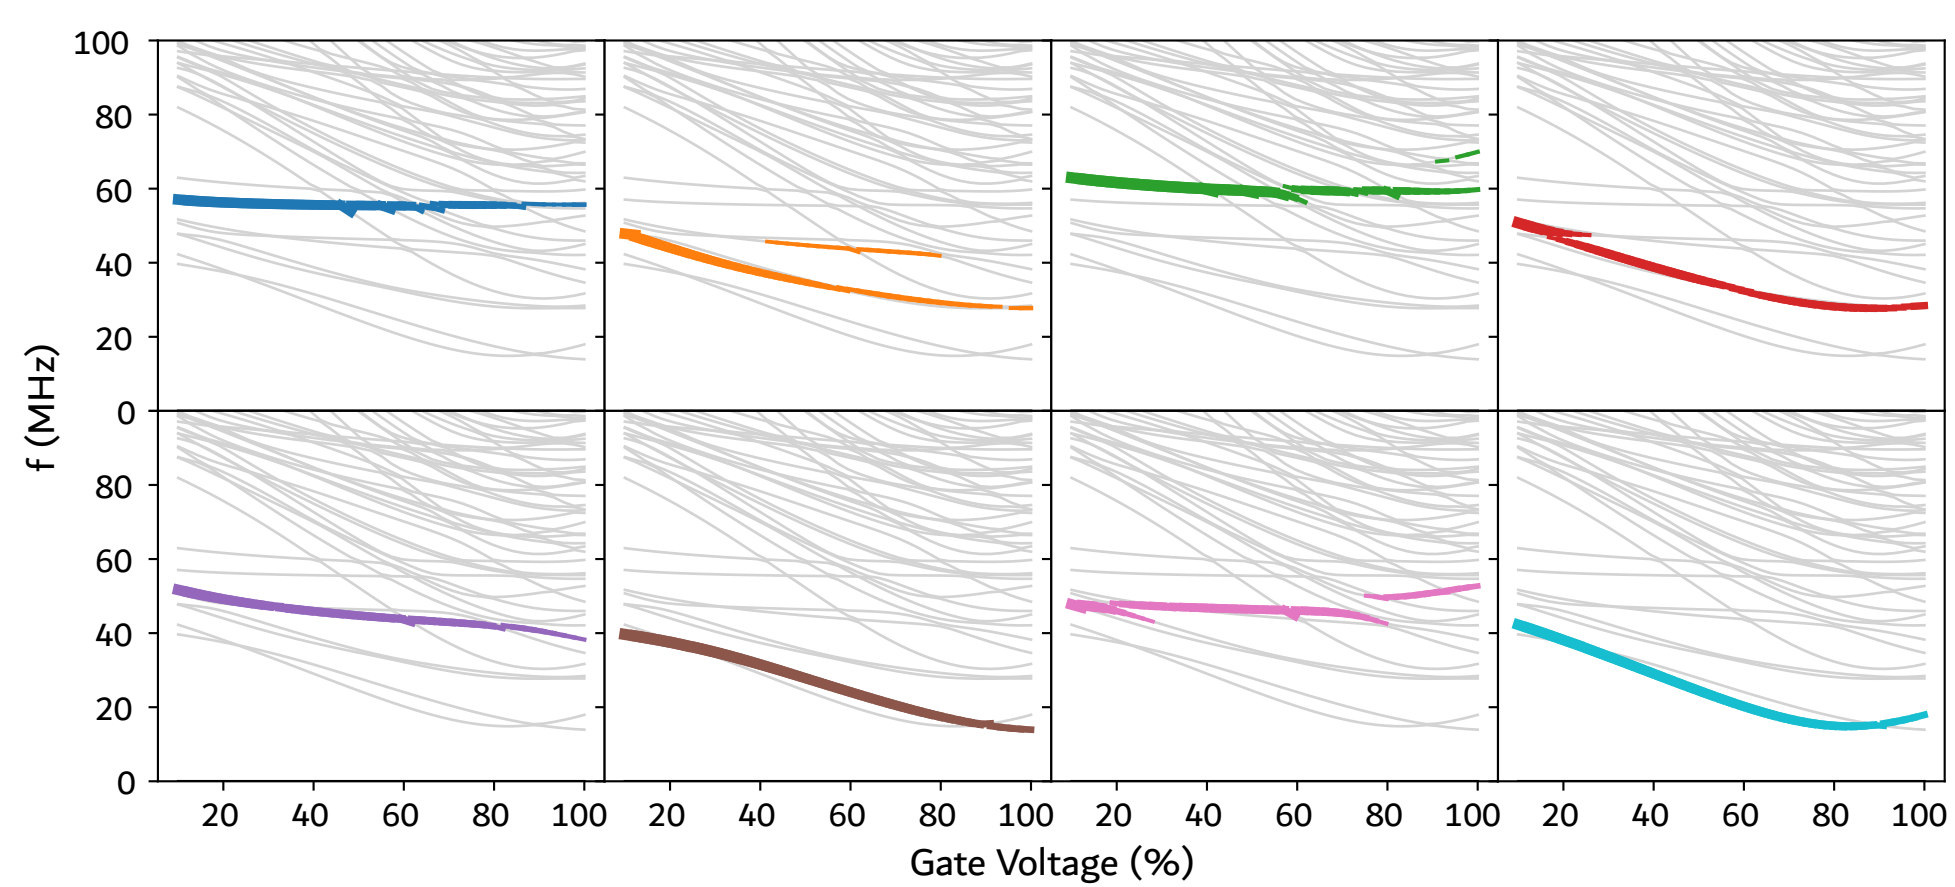

Supplement: Supplementary file 1 [file Simulated_adiabaticity.pdf]
